# Supplementary material for: DragAPart: Learning a Part-Level Motion Prior for Articulated Objects
Source: arXiv:2403.15382 source file (2024-07-28)
Supplement: Supplementary file 1 [file supmat-fig-additional-results-bg.tex]

\begin{figure}[tb!]
\includegraphics[trim={0px 0px 0px -2px}, clip, width=\linewidth]{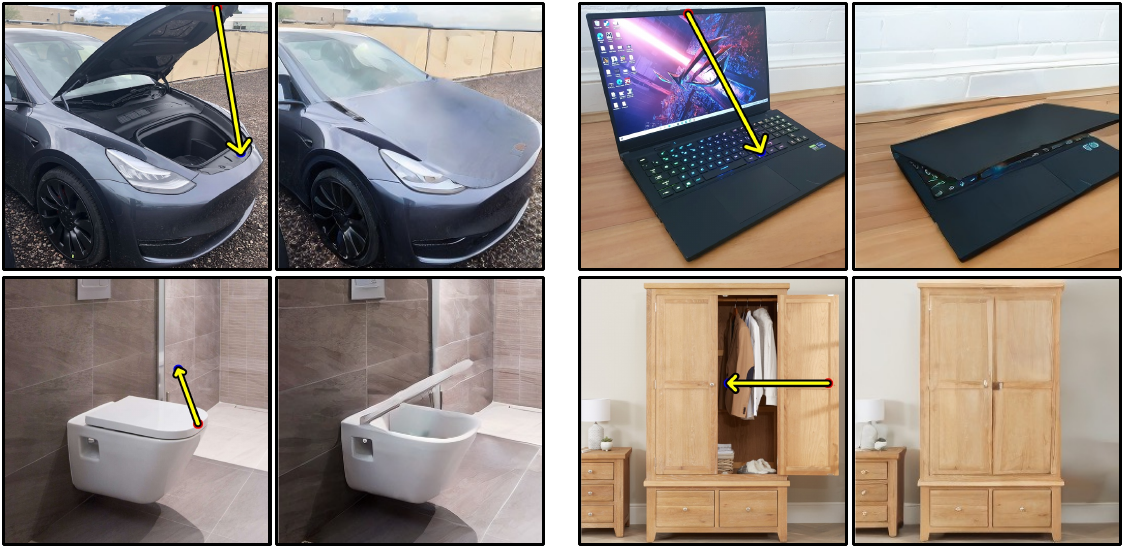}
\begin{picture}(0,0)
    \put(18,522){\scriptsize Input}
    \put(65,522){\scriptsize Generation}
    \put(137,522){\scriptsize Input}
    \put(183,522){\scriptsize Generation}
    \put(254,522){\scriptsize Input}
    \put(302,522){\scriptsize Generation}
\end{picture}
\vspace{-1.5em}
\caption{
\textbf{Additional Qualitative Results}
on images with diverse backgrounds.
}%
\label{fig:additional-results-bg}
\end{figure}
