# Supplementary material for: DragAPart: Learning a Part-Level Motion Prior for Articulated Objects
Source: arXiv:2403.15382 source file (2024-07-28)
Supplement: Supplementary file 3 [file supp-results.tex]

\section{Additional Results}
\label{sec:supp-results}

\subsection{Additional Qualitative Results}
\input{figures/supmat/supmat-fig-additional-results}
Additional results on a variety of categories can be found in \cref{fig:additional-results}.

\subsection{Failure Cases}
\input{figures/supmat/supmat-failure-cases}
We show typical failure cases of our model in \cref{fig:failure-cases}. In particular, likely due to the modest size of the training data, our model may incorrectly perceive a single part of an object as two distinct parts (left), unrealistically distort an object from an unseen category (middle), or occasionally create images that lack physical plausibility (right).

\subsection{Quantitative Comparisons on Moving Part Segmentation}
\label{sec:compare-seg}
We evaluate
